# Supplementary material for: A mechanical model of bacteriophage DNA ejection
Source: arXiv:1705.10678 source file (2017-05-30)
Supplement: Supplementary file 1 [file supplmat_pprint.tex]

\documentclass[11pt, oneside]{article}   	% use "amsart" instead of "article" for AMSLaTeX format
\usepackage{geometry}                		% See geometry.pdf to learn the layout options. There are lots.
\geometry{letterpaper}                   		% ... or a4paper or a5paper or ... 
\usepackage{graphicx}				% Use pdf, png, jpg, or eps§ with pdflatex; use eps in DVI mode
								% TeX will automatically convert eps --> pdf in pdflatex		
\usepackage{amssymb}

\title{Supplementary Material\footnote{
 \copyright 2017 This manuscript version is made available under the CC-BY-NC-ND 4.0 license http://creativecommons.org/licenses/by-nc-nd/4.0/ \hspace*{2ex}
 DOI: 10.1016/j.physleta.2017.05.044}\\
``A mechanical model of bacteriophage DNA ejection''}
\author{
Rahul Arun \& Sandip Ghosal
}
\date{}							% Activate to display a given date or no date
\begin{document}
\maketitle
\section{Photograph illustrating experimental set up}
\vspace{0.5truein}
\begin{figure}[h]
   \centering
   \includegraphics[width=1.5in]{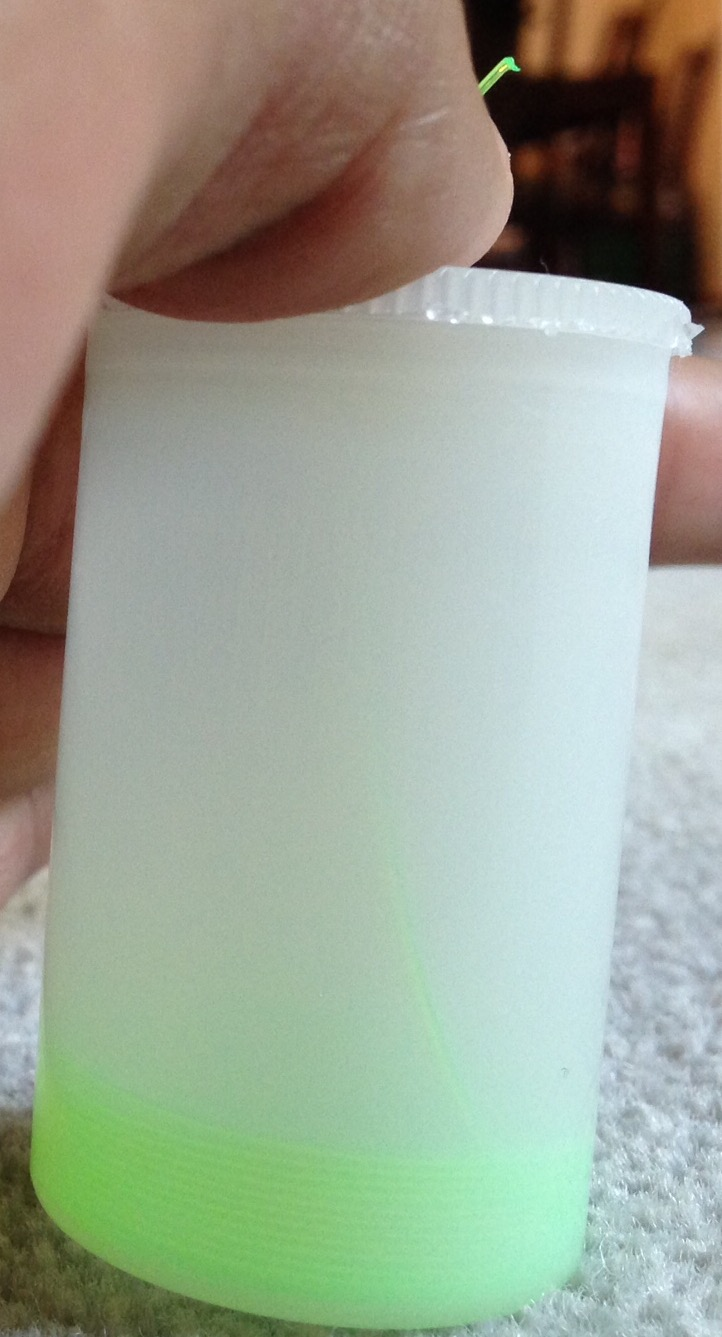} % requires the graphicx package
   \caption{Photograph of mechanical model. {\it Capsid} -- 35 mm Fuji film canister (Type: frosted clear,
   Body: HDPE, Cap: LDPE). {\it DNA} -- Nylon Monofilament fishing line, brand: Berkley Trilene Big Cat    0.022 in (0.55mm) average diameter, break strength 30 lb (13.6 kg).}
%   \label{fig:example}
\end{figure}
\newpage
\section{Video of experiment in progress}
\vspace{0.5in}
\noindent \underline{{\bf Video file}}: VideoAirSlowMo1.mov \\
(available from corresponding author upon request)\\[4ex]
\noindent \underline{{\bf Video Descriptor}}: \\[2ex]
\noindent Video of nylon monofilament with 5 cm color bands (for enhanced visibility) ejected from the film canister representing the viral capsid. The medium in this case is air. The ``Drift Innovation HD170'' Action Camera was used with a Frame Rate of 60 FPS and a resolution of 720p. The video is slowed down by a factor of 8. 
\newpage
\section{Tabular data of measured ejection times}
The data points shown in Figure~2 of the paper are as follows:
\vspace{0.25in}
\begin{table}[h]
\centering
\begin{tabular}{| c | c | } \hline
Length (cm) & Time (s) \\  \hline 
 0.0	& 0.00 \\
36.0	& 0.40\\
37.0	& 0.38\\	
37.0	& 0.41\\
37.0	& 0.43\\	
85.0	& 0.66\\	
87.0	& 0.71\\		
87.0	& 0.81\\		
90.0	& 0.86\\		
137.0 & 1.05\\		
137.0 & 1.13\\		
139.0 & 1.03\\		
139.0 & 1.13\\		
188.0 & 1.60\\		
189.0 & 1.58\\		
190.0 & 1.73\\		
200.0 & 1.96\\		
279.6 & 3.05\\		
279.6 & 3.85\\		
280.3 & 3.10\\		
 \hline
\end{tabular}
\caption{Ejected length vs time for ejections in air} 
\end{table}
\newpage
\begin{table}[h]
\centering
\begin{tabular}{| c | c | } \hline
Length (cm) & Time (s) \\  \hline 
0.0    & 	0.00\\	
36.0  & 	0.88\\
36.0  &	0.90\\
39.0  &	1.15\\
40.0  &	1.26\\
86.0  &	1.66\\
88.0  &      2.05\\		
88.0  &	2.15\\	
89.0  &	2.18\\		
135.0 &	3.32\\	
138.0 &	3.53\\		
139.0 &	3.75\\	
140.0 &	3.93\\	
186.0 &	4.63\\		
186.0 &	4.76\\		
187.0 &	4.70\\		
188.0 &    5.08\\		
261.9 &  13.01\\		
267.8 &  11.38\\	
278.0  & 13.23\\
\hline
\end{tabular}
\caption{Ejected length vs time for ejections in water} 
\end{table}
\newpage
\begin{table}[h]
\centering
\begin{tabular}{| c | c | } \hline
 Length (cm) & Time (s) \\  \hline 
 0.0	&  0.00\\
35.0  &  35.91\\
41.0  &  42.40\\
42.0  &  44.60\\
48.0	 &   54.40\\
86.0  & 100.10\\		
88.0  & 103.35\\	
92.0  & 106.63\\		
94.0  & 115.51\\		
133.0 & 125.16\\	
138.0 & 130.16\\		
138.0 & 133.65\\		
142.0 & 133.99\\		
186.0 & 272.18\\		
186.0 & 276.76\\		
187.0 & 281.21\\	
193.0 & 284.87\\		
270.1 & 670.00\\		
275.1 & 614.00\\		
276.8 & 637.00\\		
\hline
\end{tabular}
\caption{Ejected length vs time for ejections in glycerin} 
\end{table}
\end{document}
